# Supplementary material for: Towards the use of multiple ROIs for radiomics-based survival modelling: finding a strategy of aggregating lesions
Source: arXiv:2405.17668 source file (2024-12-03)
Supplement: Supplementary file 1 [file SupplementaryFIle.pdf]

Supplementary Table 1: Clinical characteristics of the study cohort. For age, median and quartiles (in brackets) are listed. For categorical variables, the number of patients and percentage (in brackets) are listed.

|                |                         | N = 115    |
|----------------|-------------------------|------------|
| Sex            | Male                    | 83 (72.2%) |
|                | Female                  | 32 (27.8%) |
| Age [Years]    |                         | 61 (57-67) |
| Histopathology | Squamous                | 77 (67.0%) |
|                | Adenocarcinoma          | 8 (7.0%)   |
|                | Not Otherwise Specified | 28 (24.3%) |
|                | Large cell              | 2 (1.7%)   |
| Location       | Left lung               | 65 (56.5%) |
|                | Right lung              | 50 (43.5%) |
| T              | 1                       | 4 (3.5%)   |
|                | 2                       | 37 (32.2%) |
|                | 3                       | 37 (32.2%) |
|                | 4                       | 37 (32.2%) |
| N              | 0                       | 19 (16.5%) |
|                | 1                       | 6 (5.2%)   |
|                | 2                       | 83 (72.2%) |
|                | 3                       | 7 (6.1%)   |
| M              | 0                       | 115 (100%) |
|                | 1                       | 0 (0%)     |
| Zubrod score   | 0                       | 34 (29.6%) |
|                | 1                       | 80 (69.6%) |
|                | 2                       | 1 (0.9%)   |

Supplementary Table 2: Summary of the performance of all schemes in MCCV on the PET dataset

| Method                   | Model        | Median c-Index | Min c-Index | Max c-Index | c-Index < 0.5 |
|--------------------------|--------------|----------------|-------------|-------------|---------------|
| MetaHistogram            | randomForest | 0.632          | 0.320       | 0.892       | 42            |
| arithmeticMeanROI        | Weibull      | 0.630          | 0.298       | 0.920       | 69            |
| arithmeticMeanROI        | CoxStepAIC   | 0.629          | 0.324       | 0.909       | 105           |
| MetaHistogram            | Weibull      | 0.625          | 0.286       | 0.868       | 72            |
| allROIMax                | Weibull      | 0.625          | 0.311       | 0.911       | 59            |
| allROIMean               | Weibull      | 0.623          | 0.267       | 0.867       | 51            |
| arithmeticMeanROI        | Loglog       | 0.620          | 0.309       | 0.867       | 64            |
| weightedMeanROI          | randomForest | 0.618          | 0.292       | 0.855       | 52            |
| allROIWeightedMean       | Weibull      | 0.617          | 0.195       | 0.843       | 70            |
| arithmeticMeanROI        | Lognormal    | 0.614          | 0.274       | 0.861       | 71            |
| allROIMean               | CoxStepAIC   | 0.614          | 0.326       | 0.878       | 83            |
| MetaHistogram            | Loglog       | 0.614          | 0.278       | 0.868       | 93            |
| largestROIdiversityIndex | randomForest | 0.613          | 0.305       | 0.890       | 74            |
| allROIMax                | randomForest | 0.613          | 0.364       | 0.890       | 91            |
| allROIMax                | Loglog       | 0.611          | 0.267       | 0.888       | 87            |
| allROIMean               | Loglog       | 0.611          | 0.284       | 0.882       | 71            |

Supplementary Table 2: Summary of the performance of all schemes in MCCV on the PET dataset

| Method                   | Model         | Median c-Index | Min c-Index | Max c-Index | c-Index < 0.5 |
|--------------------------|---------------|----------------|-------------|-------------|---------------|
| largestROI               | randomForest  | 0.611          | 0.296       | 0.862       | 75            |
| allROIWeightedMean       | Loglog        | 0.611          | 0.227       | 0.864       | 85            |
| allROIMean               | Lognormal     | 0.609          | 0.296       | 0.856       | 75            |
| allROIMax                | Lognormal     | 0.609          | 0.267       | 0.888       | 73            |
| weightedMeanROI          | Weibull       | 0.609          | 0.281       | 0.840       | 99            |
| allROIWeightedMean       | randomForest  | 0.608          | 0.322       | 0.856       | 91            |
| allROIWeightedMean       | Lognormal     | 0.607          | 0.234       | 0.838       | 83            |
| allROIMean               | randomForest  | 0.601          | 0.293       | 0.837       | 103           |
| weightedMeanROI          | Loglog        | 0.601          | 0.289       | 0.872       | 117           |
| allROIMax                | SVMvanbelle1  | 0.598          | 0.233       | 0.811       | 141           |
| weightedMeanROI          | Lognormal     | 0.596          | 0.273       | 0.872       | 124           |
| allROIMax                | SVMregression | 0.594          | 0.237       | 0.863       | 120           |
| allROIMean               | Coxnet        | 0.591          | 0.267       | 0.867       | 124           |
| allROImin                | Weibull       | 0.590          | 0.278       | 0.896       | 135           |
| allROIMax                | Coxnet        | 0.590          | 0.274       | 0.853       | 147           |
| weightedMeanROI          | CoxStepAIC    | 0.589          | 0.290       | 0.855       | 145           |
| randomROIdiversityIndex  | randomForest  | 0.589          | 0.288       | 0.846       | 136           |
| weightedMeanROI          | SVMregression | 0.588          | 0.172       | 0.873       | 153           |
| MetaHistogram            | Lognormal     | 0.588          | 0.226       | 0.890       | 158           |
| largestROI               | Loglog        | 0.587          | 0.305       | 0.848       | 150           |
| largestROI               | Lognormal     | 0.586          | 0.313       | 0.856       | 145           |
| largestROIdiversityIndex | SVMregression | 0.586          | 0.274       | 0.863       | 153           |
| allROIMax                | CoxStepAIC    | 0.586          | 0.278       | 0.890       | 174           |
| arithmeticMeanROI        | randomForest  | 0.585          | 0.276       | 0.831       | 144           |
| randomROI                | randomForest  | 0.584          | 0.295       | 0.879       | 160           |
| largestROI               | Weibull       | 0.584          | 0.313       | 0.852       | 142           |
| largestROI               | SVMregression | 0.583          | 0.244       | 0.892       | 167           |
| allROIWeightedMean       | CoxStepAIC    | 0.581          | 0.188       | 0.875       | 151           |
| MetaHistogram            | SVMvanbelle1  | 0.581          | 0.230       | 0.872       | 191           |
| allROImin                | Loglog        | 0.580          | 0.286       | 0.904       | 155           |
| allROImin                | CoxStepAIC    | 0.580          | 0.316       | 0.854       | 164           |
| largestROIdiversityIndex | Lognormal     | 0.579          | 0.303       | 0.798       | 182           |
| randomROIdiversityIndex  | Loglog        | 0.578          | 0.291       | 0.894       | 188           |
| MetaHistogram            | SVMregression | 0.578          | 0.307       | 0.908       | 195           |
| weightedMeanROI          | Coxnet        | 0.577          | 0.211       | 0.838       | 153           |
| randomROI                | Weibull       | 0.577          | 0.256       | 0.867       | 208           |
| largestROIdiversityIndex | Weibull       | 0.576          | 0.296       | 0.798       | 179           |
| randomROIdiversityIndex  | Weibull       | 0.576          | 0.260       | 0.844       | 172           |
| largestROIdiversityIndex | Loglog        | 0.576          | 0.305       | 0.826       | 179           |
| allROImin                | Lognormal     | 0.575          | 0.286       | 0.904       | 165           |
| arithmeticMeanROI        | SVMregression | 0.575          | 0.267       | 0.912       | 179           |
| allROIWeightedMean       | SVMregression | 0.575          | 0.194       | 0.873       | 198           |
| randomROIdiversityIndex  | Lognormal     | 0.574          | 0.135       | 0.907       | 198           |

Supplementary Table 2: Summary of the performance of all schemes in MCCV on the PET dataset

| Method                   | Model         | Median c-Index | Min c-Index | Max c-Index | c-Index < 0.5 |
|--------------------------|---------------|----------------|-------------|-------------|---------------|
| allROIMean               | SVMvanbelle1  | 0.572          | 0.271       | 0.872       | 207           |
| largestROI               | Coxnet        | 0.571          | 0.267       | 0.890       | 160           |
| allROIMean               | SVMregression | 0.570          | 0.267       | 0.883       | 197           |
| randomROI                | Loglog        | 0.570          | 0.281       | 0.852       | 247           |
| allROIWeightedMean       | SVMvanbelle1  | 0.569          | 0.246       | 0.841       | 248           |
| allROIWeightedMean       | Coxnet        | 0.568          | 0.230       | 0.828       | 199           |
| randomROIdiversityIndex  | SVMregression | 0.566          | 0.261       | 0.941       | 227           |
| MetaHistogram            | Coxnet        | 0.565          | 0.234       | 0.814       | 202           |
| arithmeticMeanROI        | Coxnet        | 0.565          | 0.188       | 0.844       | 169           |
| largestROIdiversityIndex | Coxnet        | 0.564          | 0.267       | 0.890       | 164           |
| randomROI                | Lognormal     | 0.563          | 0.188       | 0.920       | 264           |
| allROImin                | Coxnet        | 0.562          | 0.291       | 0.863       | 182           |
| allROImin                | randomForest  | 0.561          | 0.218       | 0.842       | 203           |
| MetaHistogram            | CoxStepAIC    | 0.556          | 0.265       | 0.897       | 134           |
| largestROI               | CoxStepAIC    | 0.554          | 0.280       | 0.880       | 268           |
| randomROI                | SVMregression | 0.553          | 0.216       | 0.902       | 288           |
| randomROIdiversityIndex  | CoxStepAIC    | 0.552          | 0.265       | 0.838       | 297           |
| randomROI                | CoxStepAIC    | 0.549          | 0.256       | 0.867       | 291           |
| largestROIdiversityIndex | CoxStepAIC    | 0.547          | 0.234       | 0.880       | 304           |
| randomROIdiversityIndex  | Coxnet        | 0.545          | 0.274       | 0.867       | 268           |
| randomROI                | Coxnet        | 0.540          | 0.246       | 0.841       | 246           |
| arithmeticMeanROI        | SVMvanbelle1  | 0.537          | 0.203       | 0.863       | 352           |
| randomROIdiversityIndex  | SVMvanbelle1  | 0.537          | 0.206       | 0.843       | 341           |
| randomROI                | SVMvanbelle1  | 0.531          | 0.237       | 0.830       | 382           |
| allROImin                | SVMregression | 0.519          | 0.187       | 0.880       | 397           |
| allROImin                | SVMvanbelle1  | 0.512          | 0.218       | 0.896       | 439           |
| weightedMeanROI          | SVMvanbelle1  | 0.487          | 0.090       | 0.778       | 553           |
| largestROI               | SVMvanbelle1  | 0.464          | 0.119       | 0.733       | 630           |
| largestROIdiversityIndex | SVMvanbelle1  | 0.456          | 0.119       | 0.776       | 671           |

Supplementary Table 3: Summary of the performance of all schemes in MCCV on the PET\_CT dataset

| Method             | Model         | Median c-Index | Min c-Index | Max c-Index | c-Index < 0.5 |
|--------------------|---------------|----------------|-------------|-------------|---------------|
| allROIMax          | randomForest  | 0.634          | 0.357       | 0.881       | 50            |
| allROIWeightedMean | randomForest  | 0.622          | 0.357       | 0.838       | 60            |
| allROIMean         | randomForest  | 0.619          | 0.316       | 0.854       | 61            |
| largestROI         | randomForest  | 0.614          | 0.309       | 0.872       | 77            |
| weightedMeanROI    | randomForest  | 0.612          | 0.288       | 0.834       | 61            |
| diversityIndexROI  | randomForest  | 0.612          | 0.300       | 0.899       | 80            |
| MetaHistogram      | Weibull       | 0.604          | 0.355       | 0.898       | 99            |
| allROIMax          | Weibull       | 0.601          | 0.349       | 0.890       | 102           |
| MetaHistogram      | Loglog        | 0.601          | 0.348       | 0.873       | 121           |
| allROIMax          | SVMregression | 0.597          | 0.249       | 0.922       | 159           |

Supplementary Table 3: Summary of the performance of all schemes in MCCV on the PET\_CT dataset

| Method                  | Model         | Median c-Index | Min c-Index | Max c-Index | c-Index < 0.5 |
|-------------------------|---------------|----------------|-------------|-------------|---------------|
| MetaHistogram           | randomForest  | 0.595          | 0.317       | 0.867       | 109           |
| largestROI              | SVMregression | 0.594          | 0.172       | 0.912       | 147           |
| MetaHistogram           | Lognormal     | 0.593          | 0.315       | 0.874       | 148           |
| weightedMeanROI         | SVMregression | 0.592          | 0.144       | 0.922       | 177           |
| randomROI               | randomForest  | 0.592          | 0.301       | 0.862       | 165           |
| diversityIndexROI       | SVMregression | 0.591          | 0.316       | 0.902       | 80            |
| randomROIdiversityIndex | randomForest  | 0.590          | 0.261       | 0.888       | 151           |
| allROIMean              | Weibull       | 0.589          | 0.341       | 0.882       | 111           |
| allROIMax               | Loglog        | 0.589          | 0.315       | 0.890       | 139           |
| allROIWeightedMean      | Weibull       | 0.588          | 0.297       | 0.824       | 128           |
| allROIWeightedMean      | SVMregression | 0.588          | 0.167       | 0.912       | 192           |
| allROIMax               | Coxnet        | 0.585          | 0.318       | 0.839       | 140           |
| allROIMean              | SVMregression | 0.584          | 0.200       | 0.912       | 217           |
| weightedMeanROI         | Weibull       | 0.583          | 0.305       | 0.840       | 147           |
| allROIMax               | Lognormal     | 0.582          | 0.315       | 0.890       | 154           |
| largestROI              | Lognormal     | 0.580          | 0.324       | 0.872       | 151           |
| allROIWeightedMean      | Loglog        | 0.580          | 0.320       | 0.824       | 144           |
| allROIMean              | Lognormal     | 0.579          | 0.311       | 0.882       | 142           |
| allROIMean              | Loglog        | 0.579          | 0.304       | 0.853       | 132           |
| largestROI              | Weibull       | 0.579          | 0.309       | 0.847       | 162           |
| allROIMax               | CoxStepAIC    | 0.579          | 0.241       | 0.847       | 178           |
| largestROI              | Loglog        | 0.578          | 0.302       | 0.881       | 175           |
| allROIMax               | SVMvanbelle1  | 0.578          | 0.255       | 0.825       | 191           |
| allROIMean              | Coxnet        | 0.578          | 0.304       | 0.853       | 136           |
| allROIWeightedMean      | Lognormal     | 0.578          | 0.305       | 0.826       | 151           |
| allROIMean              | CoxStepAIC    | 0.577          | 0.313       | 0.845       | 172           |
| allROImin               | randomForest  | 0.575          | 0.267       | 0.822       | 187           |
| weightedMeanROI         | Loglog        | 0.574          | 0.329       | 0.838       | 177           |
| weightedMeanROI         | Lognormal     | 0.573          | 0.320       | 0.825       | 181           |
| diversityIndexROI       | Lognormal     | 0.573          | 0.309       | 0.821       | 174           |
| diversityIndexROI       | Weibull       | 0.572          | 0.302       | 0.837       | 190           |
| arithmeticMeanROI       | randomForest  | 0.571          | 0.284       | 0.800       | 172           |
| MetaHistogram           | SVMregression | 0.571          | 0.296       | 0.844       | 222           |
| diversityIndexROI       | Loglog        | 0.570          | 0.309       | 0.826       | 197           |
| arithmeticMeanROI       | SVMregression | 0.569          | 0.214       | 0.902       | 258           |
| allROIWeightedMean      | Coxnet        | 0.568          | 0.296       | 0.860       | 191           |
| randomROIdiversityIndex | SVMregression | 0.567          | 0.239       | 0.873       | 147           |
| allROIWeightedMean      | CoxStepAIC    | 0.566          | 0.282       | 0.836       | 206           |
| arithmeticMeanROI       | Weibull       | 0.565          | 0.292       | 0.810       | 213           |
| allROImin               | Weibull       | 0.564          | 0.278       | 0.892       | 178           |
| allROIWeightedMean      | SVMvanbelle1  | 0.562          | 0.247       | 0.792       | 248           |
| diversityIndexROI       | Coxnet        | 0.561          | 0.281       | 0.835       | 196           |
| allROImin               | Lognormal     | 0.561          | 0.281       | 0.873       | 211           |

Supplementary Table 3: Summary of the performance of all schemes in MCCV on the PET\_CT dataset

| Method                  | Model         | Median c-Index | Min c-Index | Max c-Index | c-Index < 0.5 |
|-------------------------|---------------|----------------|-------------|-------------|---------------|
| allROImin               | Loglog        | 0.561          | 0.263       | 0.863       | 204           |
| weightedMeanROI         | CoxStepAIC    | 0.559          | 0.309       | 0.873       | 243           |
| largestROI              | Coxnet        | 0.559          | 0.259       | 0.790       | 178           |
| allROImin               | SVMregression | 0.557          | 0.167       | 0.878       | 299           |
| allROImin               | CoxStepAIC    | 0.556          | 0.263       | 0.859       | 255           |
| allROImin               | Coxnet        | 0.555          | 0.245       | 0.863       | 212           |
| weightedMeanROI         | Coxnet        | 0.554          | 0.266       | 0.847       | 177           |
| arithmeticMeanROI       | CoxStepAIC    | 0.554          | 0.308       | 0.786       | 252           |
| arithmeticMeanROI       | Loglog        | 0.553          | 0.280       | 0.816       | 243           |
| randomROIdiversityIndex | Weibull       | 0.552          | 0.193       | 0.848       | 287           |
| randomROI               | SVMregression | 0.552          | 0.161       | 0.859       | 300           |
| arithmeticMeanROI       | Lognormal     | 0.551          | 0.281       | 0.776       | 241           |
| MetaHistogram           | SVMvanbelle1  | 0.550          | 0.200       | 0.832       | 290           |
| allROImin               | SVMvanbelle1  | 0.549          | 0.240       | 0.800       | 304           |
| randomROI               | SVMvanbelle1  | 0.545          | 0.235       | 0.846       | 316           |
| randomROIdiversityIndex | SVMvanbelle1  | 0.543          | 0.147       | 0.853       | 334           |
| randomROI               | Loglog        | 0.541          | 0.293       | 0.856       | 317           |
| arithmeticMeanROI       | Coxnet        | 0.540          | 0.282       | 0.826       | 255           |
| largestROI              | CoxStepAIC    | 0.540          | 0.262       | 0.908       | 313           |
| diversityIndexROI       | CoxStepAIC    | 0.539          | 0.262       | 0.908       | 323           |
| randomROIdiversityIndex | Loglog        | 0.539          | 0.269       | 0.839       | 312           |
| randomROI               | Weibull       | 0.539          | 0.302       | 0.875       | 322           |
| MetaHistogram           | Coxnet        | 0.536          | 0.222       | 0.831       | 283           |
| randomROIdiversityIndex | Lognormal     | 0.535          | 0.280       | 0.815       | 336           |
| randomROI               | CoxStepAIC    | 0.535          | 0.196       | 0.892       | 350           |
| randomROIdiversityIndex | CoxStepAIC    | 0.534          | 0.234       | 0.805       | 332           |
| randomROI               | Lognormal     | 0.534          | 0.224       | 0.806       | 366           |
| MetaHistogram           | CoxStepAIC    | 0.534          | 0.261       | 0.845       | 226           |
| arithmeticMeanROI       | SVMvanbelle1  | 0.523          | 0.245       | 0.825       | 412           |
| randomROI               | Coxnet        | 0.521          | 0.167       | 0.781       | 285           |
| randomROIdiversityIndex | Coxnet        | 0.516          | 0.273       | 0.853       | 285           |
| weightedMeanROI         | SVMvanbelle1  | 0.515          | 0.062       | 0.762       | 434           |
| largestROI              | SVMvanbelle1  | 0.507          | 0.090       | 0.775       | 467           |
| allROImin               | SVMvanbelle1  | 0.504          | 0.183       | 0.816       | 477           |
| diversityIndexROI       | SVMvanbelle1  | 0.498          | 0.096       | 0.783       | 504           |
